# Supplementary material for: A Fast Parallel Median Filtering Algorithm Using Hierarchical Tiling
Source: arXiv:2507.19926 ancillary file (2025-07-26)
Supplement: Supplementary file 1 [file supplemental_material.pdf]

# A Fast Parallel Median Filtering Algorithm Using Hierarchical Tiling - Supplemental Material

LOUIS SUGY, NVIDIA, Germany

## 1 FULL ALGORITHM PSEUDO-CODE

This section translates the algorithm described textually in the main paper to code. It is complementary to the paper and aims to facilitate reproduction of the method.

Let us first define, in Algorithm 1, a structure containing all data associated with a tile as well as useful constants<sup>1</sup>. When going down one level of the recursion, we create two such child structures for each parent structure.

### ALGORITHM 1: Tile data structure

```
struct TileData(KernelW, KernelH, TileW, TileH)
  const CoreW  $\leftarrow$  KernelW - (TileW - 1)
  const CoreH  $\leftarrow$  KernelH - (TileH - 1)
  const NumExtraCols  $\leftarrow$  2 * (TileW - 1)
  const NumExtraRows  $\leftarrow$  2 * (TileH - 1)
  const Remaining  $\leftarrow$  (TileW - 1) * CoreH + (TileH - 1) * CoreW +
    (TileW - 1) * (TileH - 1)
  const SortedCoreSize  $\leftarrow$  min(CoreW * CoreH, Remaining + 1)

  var sortedCore[SortedCoreSize]
  var extraCols[NumExtraCols, CoreH]
  var extraRows[NumExtraRows, CoreW]
  var corners[NumExtraRows, NumExtraCols]
  var medians[TileH, TileW]
```

The recursion is based on two operations: horizontal and vertical splits. This is where most of the computations happen. We will assume that we have functions to sort a list, and merge two or more lists while discarding extrema. The horizontal split is described in Algorithm 2, using NumPy-style array slicing syntax. The vertical split can be obtained by transposition (switch rows/cols and width/height).

The recursion is described in Algorithm 3. It splits the tile either horizontally or vertically, until reaching the leaf tile size.

The full median filter for one root tile is given in Algorithm 4. For simplicity, we assume that the image size is a multiple of the tile size, to omit boundary conditions. We also omit optimizations such as shared column sorting for multiple tiles. The algorithm starts with an initialization step filling the root tile data structure, followed by the recursion.

<sup>1</sup>Those would typically be compile-time constant expressions when compiling the algorithm for each kernel/tile configurations.

Author's address: Louis Sugy, NVIDIA, Munich, Germany.

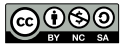

This work is licensed under a Creative Commons Attribution-NonCommercial-ShareAlike 4.0 International License.

### ALGORITHM 2: Horizontal split

```
function HORIZONTALSPLIT(tile : TileData)  $\rightarrow$  TileData[2]
  var childTiles : TileData[2]
  for iChild  $\leftarrow$  0 to 1
    var childTile  $\leftarrow$  TileData(tile.KernelW, tile.KernelH,
      tile.TileW / 2, tile.TileH)

    Merge columns to the sorted core, discard extrema
    var colStart  $\leftarrow$  (tile.TileW / 2) * (iChild + 1) - 1
    var colEnd  $\leftarrow$  colStart + tile.TileW / 2
    var newCols  $\leftarrow$  tile.extraCols[colStart : colEnd, :]
    var mergedCols  $\leftarrow$  MULTIWAYMERGE(newCols)
    childTile.sortedCore  $\leftarrow$  MERGEANDCROP(tile.sortedCore,
      mergedCols)

    Merge corners to the extra rows
    for iRow  $\leftarrow$  0 to tile.NumExtraRows - 1
      var newElts  $\leftarrow$  tile.corners[iRow, colStart : colEnd]
      var sortedElts  $\leftarrow$  SORT(newElts)
      childTile.extraRows[iRow]  $\leftarrow$  MERGE(
        tile.extraRows[iRow], sortedElts)

    Copy remaining columns and corners
    for iSide  $\leftarrow$  0 to 1
      var srcColStart  $\leftarrow$  (tile.TileW / 2) * iChild + (tile.TileW -
        1) * iSide
      var srcColEnd  $\leftarrow$  srcColStart + childTile.TileW - 1
      var dstColStart  $\leftarrow$  (childTile.TileW - 1) * iSide
      var dstColEnd  $\leftarrow$  dstColStart + childTile.TileW - 1
      childTile.extraCols[dstColStart : dstColEnd, :]  $\leftarrow$ 
        tile.extraCols[srcColStart : srcColEnd, :]
      childTile.corners[:, dstColStart : dstColEnd]  $\leftarrow$ 
        tile.corners[:, srcColStart : srcColEnd]

    childTiles[iChild]  $\leftarrow$  childTile

  return childTiles
```

### ALGORITHM 3: Recursion

```
function RECURSION(tile : TileData)
  if tile.TileW = 1 and tile.TileH = 1
    tile.medians[0][0]  $\leftarrow$  tile.sortedCore[0]
    return
  if tile.TileW  $\geq$  tile.TileH
    var childTiles  $\leftarrow$  HORIZONTALSPLIT(tile)
    for iChild  $\leftarrow$  0 to 1
      RECURSION(childTiles[iChild])
      tile.medians[:, (tile.TileW / 2) * iChild : (tile.TileW / 2) *
        (iChild + 1)]  $\leftarrow$  childTiles[iChild].medians[:, :]
  else
    var childTiles  $\leftarrow$  VERTICALSPLIT(tile)
    for iChild  $\leftarrow$  0 to 1
      RECURSION(childTiles[iChild])
      tile.medians[(tile.TileH / 2) * iChild : (tile.TileH / 2) *
        (iChild + 1), :]  $\leftarrow$  childTiles[iChild].medians[:, :]
```

**ALGORITHM 4:** Full median filter for one root tile

---

```

function MEDIANFILTER(KernelW, KernelH, TileW, TileH, imgIn,
imgOut, tileX, tileY)
  const FootprintW  $\leftarrow$  KernelW + TileW - 1
  const FootprintH  $\leftarrow$  KernelH + TileH - 1

  var x0  $\leftarrow$  TileW * tileX
  var y0  $\leftarrow$  TileH * tileY
  var tile  $\leftarrow$  TileData(KernelW, KernelH, TileW, TileH)

  Load input tile footprint
  var offsetX  $\leftarrow$  x0 - (KernelW - 1) / 2
  var offsetY  $\leftarrow$  y0 - (KernelH - 1) / 2
  var footprint  $\leftarrow$  imgIn[offsetY : offsetY + FootprintH, offsetX :
offsetX + FootprintW]

  Sort core columns and extra columns
  for iCol  $\leftarrow$  0 to FootprintW - 1
  | footprint[TileH - 1 : TileH - 1 + tile.CoreH, iCol]  $\leftarrow$  SORT(
  | footprint[TileH - 1 : TileH - 1 + tile.CoreH, iCol])

  Sort core by merging sorted core columns, discard extrema
  tile.sortedCore  $\leftarrow$  MULTIWAYMERGEANDCROP(footprint[TileH -
1 : TileH - 1 + tile.CoreH, TileW - 1 : TileW - 1 + tile.CoreW])

  Copy sorted extra columns
  for iLR  $\leftarrow$  0 to 1
  | tile.extraCols[(TileW - 1) * iLR : (TileW - 1) * (iLR + 1), :]  $\leftarrow$ 
  | TRANSPOSE(footprint[TileH - 1 : TileH - 1 + tile.CoreH,
  | KernelW * iLR : KernelW * iLR + TileW - 1])

  Sort and copy extra rows
  for iTB  $\leftarrow$  0 to 1
  | for iRow  $\leftarrow$  0 to TileH - 1
  | | tile.extraRows[(TileH - 1) * iTB + iRow, :]  $\leftarrow$ 
  | | SORT(footprint[KernelH * iTB + iRow, TileW - 1 :
  | | TileW - 1 + tile.CoreW])

  Copy corners
  for iLR  $\leftarrow$  0 to 1
  | for iTB  $\leftarrow$  0 to 1
  | | tile.corners[(TileH - 1) * iTB : (TileH - 1) * (iTB + 1),
  | | (TileW - 1) * iLR : (TileW - 1) * (iLR + 1)]  $\leftarrow$ 
  | | footprint[KernelH * iTB : KernelH * iTB + TileH - 1,
  | | KernelW * iLR : KernelW * iLR + TileW - 1]

  Start recursion from the root tile
  RECURSION(tile)

  Write medians to the output image
  imgOut[y0 : y0 + TileH, x0 : x0 + TileW]  $\leftarrow$  tile.medians[:, :]

```

---

## 2 EXCLUSION OF EXTREMA

One detail that has been abstracted away in the above pseudo-code is the specific math behind the exclusion of extrema.

For a  $k \times k$  kernel, we are finding the median of  $k^2$  elements, which is an odd number. Let us define  $r = \lfloor \frac{k^2}{2} \rfloor = \frac{k^2-1}{2}$ . The median is at the index  $r$  of the full sorted kernel.

We also name  $n_s$  the number of elements that were previously excluded as smaller than the median,  $n_g$  the number of elements that were excluded as greater than the median,  $m$  the number of unseen elements, and  $p$  the number of elements that we have seen and sorted but not yet excluded. By definition,  $n_s + n_g + m + p = k^2$ .

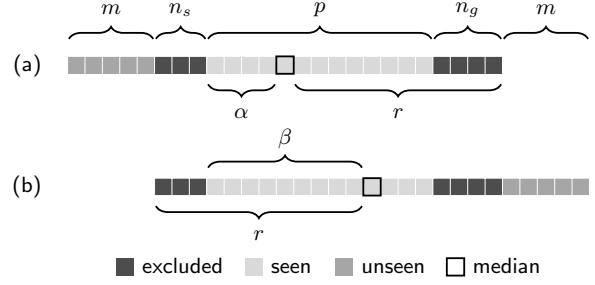

Fig. 1. Illustration of the formula for  $\alpha$  and  $\beta$ . We consider two extreme scenarios where: (a) all unseen elements are smaller than all elements seen so far; (b) all unseen elements are greater.

We wish to find  $\alpha$  and  $\beta$ , the first and last (inclusive) indices of elements, in the current list of size  $p$ , that are potential median candidates. Considering the extreme cases where the unseen elements are smaller than all seen elements, or greater than all seen elements, we find that:

$$\alpha = \max(0, p + n_g - r - 1)$$

$$\beta = \min(p - 1, r - n_s)$$

This is best explained visually, in Figure 1.

If less than half of the elements are unseen, the number of elements remaining after the exclusion of extrema is  $\beta - \alpha + 1 = 2r + 1 - p - n_s - n_g + 1 = m + 1$ . This corresponds to the principle of forgetfulness described in the paper.

## 3 ANALYSIS

### 3.1 Data-oblivious variant

**3.1.1 Networks.** We aim to build a data-oblivious sorting network. All the networks that are used as building blocks must satisfy that constraint. We ignore data-oblivious sorting networks with  $O(n \log(n))$  complexity that are not practical to use due to large constant factors, such as Goodrich's zig-zag sorting network [2014]. Based on Batchier and Lee's analysis [1968] [1995] that can be extended to non-powers of two by padding up to the next power of two with a large value, we know upper bounds on the complexity of the following networks:

**Sorting network** for a list of size  $n$ :  $O(n \log(n)^2)$ .

**Merging network** for two sorted lists of sizes  $p$  and  $q$ :  $O((p + q) \log(p + q))$ .

**Multi-way merging network** for  $k$  sorted lists of size  $n$ :  $O(kn \log(k) \log(n))$ .

**3.1.2 Complexity.** Let  $k$  be an odd integer,  $k \geq 3$ . We show that the per-pixel number of operations of a  $k \times k$  median filter using our hierarchical separable sorting network has a complexity  $O(k \log(k))$ .

**PROOF.** Let us define the following heuristic to choose root tile dimensions that grow linearly with the kernel diameter  $k$ :

$$t_w^{(0)} = t_h^{(0)} = t(k) = 2^{\lfloor \log_2(k) \rfloor - 1}$$

The core of the root tile is of dimensions  $c_w^{(0)} \times c_h^{(0)}$  which can also be expressed as a function of  $k$ :

$$c_w^{(0)} = c_h^{(0)} = c(k) = k - t(k) + 1$$

We find the following relations:

$$\frac{k}{4} < t(k) < \frac{k}{2} \quad \text{so } t(k) = \Theta(k) \quad (1)$$

$$c(k) \leq k \quad \text{so } c(k) = O(k) \quad (2)$$

Let us first consider the stages executed only for the root tile.

- Sort columns: We sort on average  $t_w^{(0)}$  columns of height  $c_h^{(0)}$  for each root tile. The cost per tile, simplified using equations 1 and 2, is:

$$O\left(t(k)c(k)\log(c(k))^2\right) = O\left(k^2\log(k)^2\right)$$

- Sort core: We use a multi-way merging network of  $c_w^{(0)}$  lists of length  $c_h^{(0)}$ . The cost per tile is:

$$O\left(c(k)^2\log(c(k))^2\right) = O\left(k^2\log(k)^2\right)$$

- Sort extra rows: We sort  $2(t_h^{(0)} - 1)$  rows of width  $c_w^{(0)}$ . The cost per tile is:

$$O\left(t(k)c(k)\log(c(k))^2\right) = O\left(k^2\log(k)^2\right)$$

We now consider the stages of splitting a  $t_w^{(i)} \times t_h^{(i)}$  parent tile horizontally. The following operations are executed for each of the two child tiles:

- Merge extra columns together: We merge  $t_w^{(i)}/2$  columns of height  $c_h^{(i)} \leq k$ . The cost is:

$$O\left(t_w^{(i)}k\log\left(t_w^{(i)}\right)\log(k)\right)$$

- Merge extra columns with the sorted core: The number of elements selected from the sorted core is defined by the number of inputs that remain to be merged. It is bounded by  $k(t_w^{(i)} + t_h^{(i)})$ . The number of elements in the columns to be merged is  $(t_w^{(i)}/2)c_h^{(i)}$ , with  $c_h^{(i)} \leq k$ . The cost is:

$$O\left(k\left(t_w^{(i)} + t_h^{(i)}\right)\log\left(k\left(t_w^{(i)} + t_h^{(i)}\right)\right)\right)$$

- Sort groups of corners: For each of  $2(t_h^{(i)} - 1)$  extra rows, we need to sort  $t_w^{(i)}/2$  corners. The cost is:

$$O\left(t_h^{(i)}t_w^{(i)}\log\left(t_w^{(i)}\right)^2\right)$$

- Merge corners with extra rows: For each of  $2(t_h^{(i)} - 1)$  extra rows, we need to merge  $c_w^{(i)} \leq k$  elements from the row and  $t_w^{(i)}/2 < k$  corners. The cost is:

$$O\left(t_h^{(i)}k\log(k)\right)$$

The cost of each stage of the vertical split is found similarly, substituting  $t_h^{(i)}$  for  $t_w^{(i)}$  and vice versa.

We start with a square tile, so a horizontal split followed by a vertical split results in a smaller square tile, and so on. We can express the tile dimensions at even depths of the recursion as:

$$t_w^{(2i)} = t_h^{(2i)} = \frac{t(k)}{2^i}$$

Adding up the costs of all stages of the horizontal split and vertical split for all child tiles, we find that the cost of splitting a square tile  $t_h^{(2i)} \times t_w^{(2i)}$  into four  $t_h^{(2(i+1))} \times t_w^{(2(i+1))}$  tiles is:

$$O\left(\frac{t(k)}{2^i}k\log\left(\frac{t(k)}{2^i}\right)\log(k)\right)$$

To compute the total cost of the recursion for each root tile, we sum up the costs for all the tiles at each level:

$$\begin{aligned} & O\left(\sum_{i=0}^{\log_2(t(k))-1} 2^{2i} \frac{t(k)}{2^i} k \log\left(\frac{t(k)}{2^i}\right) \log(k)\right) \\ &= O\left(t(k)k\log(k) \sum_{i=0}^{\log_2(t(k))-1} 2^i (\log(t(k)) - i)\right) \\ &= O\left(t(k)^2k\log(k)\right) \end{aligned}$$

We finally add up the cost of the initial stages and the cost of the recursion, divide the total by the number of pixels per root tile, and simplify using equation 1, to obtain the cost per pixel:

$$O\left(\frac{k^2\log(k)^2 + t(k)^2k\log(k)}{t(k)^2}\right) = O(k\log(k))$$

□

## 3.2 Data-aware variant

**3.2.1 Sorting and merging.** In the paper, we described several algorithms for parallel merging and sorting. Although we know linear algorithms for such operations, the complexities of the algorithms that we use in our implementation are sufficient assumptions to prove the linear complexity of the broader algorithm:

**Sorting network** for a list of size  $n$ :  $O(n\log(n)^2)$ .

**Merging** two sorted lists of sizes  $p$  and  $q$ :  $O(p + q)$ .

**Multi-way merging**  $k$  sorted lists of size  $n$ :  $O(kn\log(k))$ .

**3.2.2 Complexity.** Let  $k$  be an odd integer,  $k \geq 3$ . The per-pixel complexity of a  $k \times k$  median filter using the hierarchical-tiling median filtering algorithm is  $O(k)$ .

**PROOF.** Using the heuristic introduced in Section 3.1.2, and relations 1 and 2, we follow the same steps, substituting the complexities of data-oblivious operations with their data-aware counterparts when relevant. In particular, we focus on the recursion which dominates the complexity.

Let us consider the stages of splitting a  $t_w^{(i)} \times t_h^{(i)}$  parent tile horizontally. The following operations are executed for each of the two child tiles:

- Merge extra columns. The updated cost is:

$$O\left(t_w^{(i)}k\log\left(t_w^{(i)}\right)\right)$$

- Merge extra columns with the sorted core. The updated cost is:

$$O\left(k\left(t_w^{(i)} + t_h^{(i)}\right)\right)$$

- Sort groups of corners. The cost is still:

$$O\left(t_h^{(i)}t_w^{(i)}\log\left(t_w^{(i)}\right)^2\right)$$

- Merge corners with extra rows. The updated cost is:

$$O\left(t_h^{(i)} k\right)$$

Adding up the costs of all stages of the horizontal split and vertical split for all child tiles, we now find that the cost of splitting a square tile  $t_h^{(2i)} \times t_w^{(2i)}$  into four  $t_h^{(2(i+1))} \times t_w^{(2(i+1))}$  tiles is:

$$O\left(\frac{t(k)}{2^i} k \log\left(\frac{t(k)}{2^i}\right) + \left(\frac{t(k)}{2^i}\right)^2 \log\left(\frac{t(k)}{2^i}\right)^2\right)$$

To compute the total cost of the recursion for each root tile, we sum up the costs for all the tiles at each level:

$$\begin{aligned} & O\left(\sum_{i=0}^{\log_2(t(k))-1} 2^{2i} \left(\frac{t(k)}{2^i} k \log\left(\frac{t(k)}{2^i}\right) + \left(\frac{t(k)}{2^i}\right)^2 \log\left(\frac{t(k)}{2^i}\right)^2\right)\right) \\ &= O\left(\sum_{i=0}^{\log_2(t(k))-1} 2^i t(k) k (\log(t(k)) - i) + t(k)^2 \log\left(\frac{t(k)}{2^i}\right)^2\right) \\ &= O\left(\sum_{i=0}^{\log_2(t(k))-1} 2^i t(k) k (\log(t(k)) - i) + t(k)^2 \frac{t(k)}{2^i}\right) \\ &= O\left(t(k)^2 k + t(k)^3\right) \\ &= O\left(t(k)^2 k\right) \end{aligned}$$

Once more, we add up the cost of the initial stages and the cost of the recursion, divide the total by the number of pixels per root tile, and simplify to obtain the cost per pixel:

$$O\left(\frac{k^2 \log(k)^2 + t(k)^2 k}{t(k)^2}\right) = O(k)$$

□

## 4 COMPILATION TIMES

As mentioned in the paper, the data-oblivious version of our method needs to be compiled for each combination of parameters (kernel and tile size), as each combination uses a different selection network. For performance reasons, the data-aware implementation also contains template-specialized functions that are instantiated multiple times.

Our test and benchmark cover 8-bit and 16-bit integers, and 32-bit floating-point numbers, with all the square kernel sizes from  $3 \times 3$  to  $31 \times 31$  for the data-oblivious variant, and from  $3 \times 3$  to  $75 \times 75$  for the data-aware variant. We measured around 8 minutes of compilation time for each variant, including all these combinations of parameters. The generation of all the sorting networks with a Python script is almost negligible, taking less than a second.

The compilation times of the data-oblivious variant, for each data type and kernel size, are detailed in Figure 2.

We observe that compilation times rapidly increase for  $13 \times 13$  and above, at the point where this implementation starts suffering from register pressure and local memory spilling. It is also interesting to note a difference in compilation times between data types: the smaller data types have longer compilation times, despite using essentially the same code at the CUDA C++ level. Indeed, the compiler front-end takes approximately the same time, but most of the

compilation time is spent between the optimization of the NVVM IR and the final compilation from PTX to SASS.

We cannot separate the compilation time of the data-aware version per kernel size in the same way, as most functions are not compiled specifically for one kernel size; thus, compiling all combinations is significantly faster than compiling for each kernel size independently.

## 5 MEMORY USAGE

### 5.1 Data-oblivious variant

The data-oblivious variant requires no additional allocation besides the input and output data. For small kernel sizes, all intermediate data is in registers and shared memory.

However, for larger kernel sizes, register pressure causes the compiler to spill to local memory, which is backed by DRAM. The amount of memory reserved for local memory spills does not depend on the input resolution, but on the maximum number of threads that can execute on this GPU, so it scales with the number of Streaming Multiprocessors. On a GPU with many SMs like L40S, it reaches up to 1.8 GiB for a  $31 \times 31$  kernel.

### 5.2 Data-aware variant

The data-aware variant allocates buffers for intermediate data. The size of the allocation scales linearly with the number of pixels, the kernel diameter, and the data type size.

If we execute the median filter over the entire image at once, the buffer allocations can exceed the size of the input image by two orders of magnitude. For instance, filtering a 30-megapixel image in 32-bit precision would require up to 25 GiB of memory.

However, the filter can be applied iteratively to rectangular regions of the image to meet an arbitrary memory budget. An appropriate slice size can also significantly increase the throughput, as the intermediate buffers suffer from less cache thrashing. The memory usage and throughput with and without slicing are compared in Figure 3.

## REFERENCES

- K. E. Batchier. 1968. Sorting networks and their applications. In *Proceedings of the April 30–May 2, 1968, Spring Joint Computer Conference* (Atlantic City, New Jersey) (AFIPS '68 (Spring)). Association for Computing Machinery, New York, NY, USA, 307–314. <https://doi.org/10.1145/1468075.1468121>
- Michael T. Goodrich. 2014. Zig-zag sort: a simple deterministic data-oblivious sorting algorithm running in  $O(n \log n)$  time. In *Proceedings of the Forty-Sixth Annual ACM Symposium on Theory of Computing* (New York, New York) (STOC '14). Association for Computing Machinery, New York, NY, USA, 684–693. <https://doi.org/10.1145/2591796.2591830>
- De-Lei Lee and K.E. Batchier. 1995. A multiway merge sorting network. *IEEE Transactions on Parallel and Distributed Systems* 6, 2 (1995), 211–215. <https://doi.org/10.1109/71.342136>

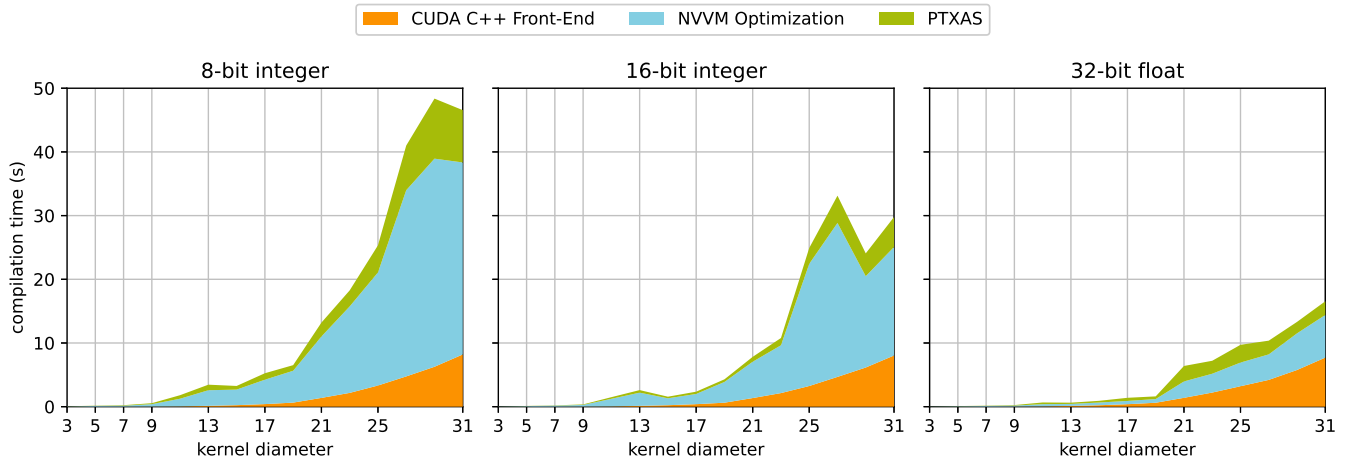

Fig. 2. Compilation time per stage for the data-oblivious variant of our method, for various data types and kernel sizes.

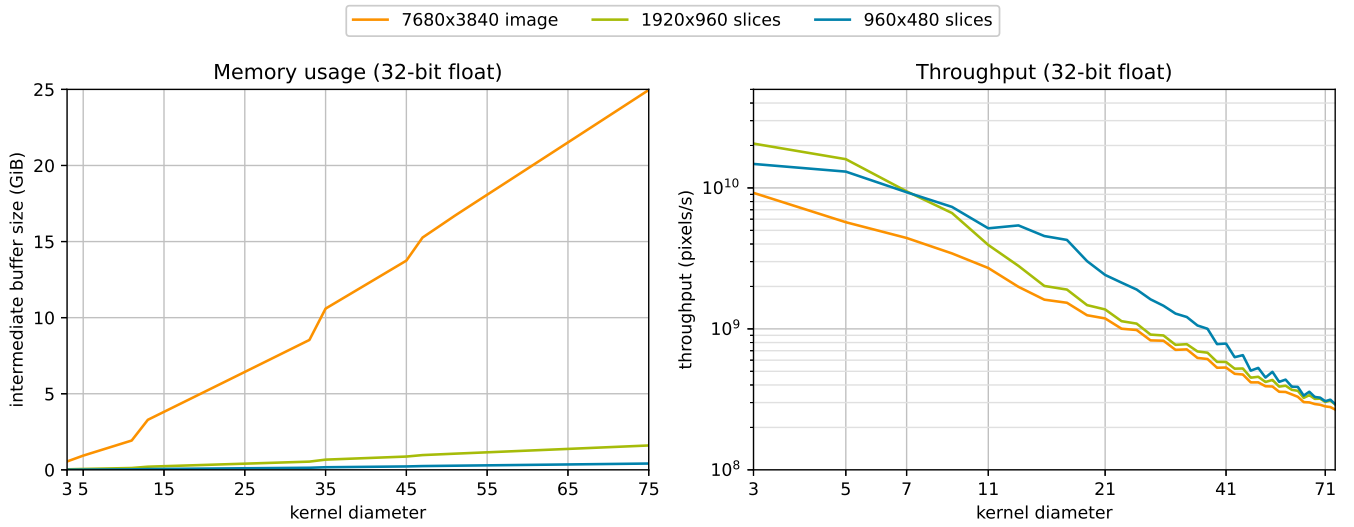

Fig. 3. Size of the intermediate buffers and throughput, for the median filter applied to the entire 7680 × 3840 image at once, versus iteratively over 1920 × 960 or 960 × 480 slices. Slicing results in much lower memory requirements and better performance.
